# Supplementary material for: Locality-based Graph Reordering for Processing Speed-Ups and Impact of Diameter
Source: arXiv:2111.12281 source file (2022-02-03)
Supplement: Supplementary file 1 [file Appendix_1.tex]

\clearpage
\section{Appendix}
\label{app:A}

\subsection{}
